# Supplementary material for: Exploring the Distinctive Tweeting Patterns of Toxic Twitter Users
Source: arXiv:2401.14141 source file (2024-01-25)
Supplement: Supplementary file 1 [file appendix.tex]

\section{Appendix}
\label{}
These two tables elaborate the yearly activity spans of the Gantt charts~\ref{fig:newplot.png}, and~\ref{fig:newplot(1).png} in Section~\ref{sec:comparison}. \textcolor{blue}{add a reference in section 4.4 if the paper has enough space, or else, remove the appendix.}
\begin{table}[]
\centering
\resizebox{0.50\textwidth}{!}{
{\large
\begin{tabular}{l|r|r}
\toprule
{\bf \#years}& {\bf \#timelines}&{\bf \# users}\\
\midrule
%%%%%%%%7777
1& [2021]&3(0.20\%)\\\hline 
1& [2020]&119(8.16\%)\\\hline 
1& [2019]& 16(1.09\%)\\\hline 
1& [2018]& 7(0.48\%)\\\hline 
1& [2017]& 13(0.89\%)\\\hline 
1& [2016]& 1(0.06\%)\\\hline 
2&  [2020, 2021]& 39(2.67\%) \\\hline
2& 	[2019, 2020]& 39(2.67\%) \\\hline
2& 	[2018, 2019]& 5(0.34\%)\\\hline
2& [2017, 2019]&1(0.06\%)\\\hline
2& [2017, 2018]& 10(0.68\%) 	\\\hline
2& [2016, 2017]& 3(0.20\%) \\\hline
3&[2015, 2016, 2017]& 	3(0.20\%) \\\hline
3&[2018, 2019, 2020] &	29(1.99\%)\\\hline
3&[2017, 2018, 2020]& 	2(0.13\%) \\\hline
3&[2017, 2018, 2019]&	3(0.20\%)\\\hline
3&[2016, 2017, 2018]& 	18(1.23\%)\\\hline
3&[2019, 2020, 2021]& 	261(17.91\%)\\\hline
4&[2018, 2019, 2020, 2021]& 	149(10.22\%)\\\hline
4&[2017, 2018, 2019, 2020]& 	13(0.89\%)\\\hline
4&[2016, 2017, 2018, 2019]& 	2(0.13\%)\\\hline
4&[2015, 2016, 2017, 2018]& 	4(0.27\%)\\\hline
4&[2012, 2019, 2020, 2021]& 	1(0.06\%)\\\hline
5&[2017, 2018, 2019, 2020, 2021]& 	100(6.86\%) \\\hline
5&[2016, 2017, 2018, 2019, 2020]& 	8(0.54\%)\\\hline
6&[2014, 2015, 2016, 2017, 2018, 2019]& 	1(0.06\%)\\\hline
6&[2015, 2016, 2017, 2018, 2019, 2020]& 	5(0.34\%)\\\hline
6&[2016, 2017, 2018, 2019, 2020, 2021]& 	44(3.01\%)\\\hline
7&[2012, 2016, 2017, 2018, 2019, 2020, 2021]&	1(0.06\%) \\\hline
7&[2014, 2015, 2016, 2017, 2018, 2019, 2020]& 	1(0.06\%) 	\\\hline
7&[2015, 2016, 2017, 2018, 2019, 2020, 2021]& 	24(1.64\%)\\\hline
8&[2014, 2015, 2016, 2017, 2018, 2019, 2020, 2021]& 	12(0.82\%)\\\hline
8&[2013, 2014, 2015, 2016, 2017, 2018, 2019, 2020]& 	5(0.34\%)\\\hline
9&[2013, 2014, 2015, 2016, 2017, 2018, 2019, 2020,2021]& 	3(0.20\%)\\\hline
9&[2012, 2013, 2014, 2015, 2016, 2017, 2018, 2019, 2020]&	5(0.34\%)\\\hline
10&[2011, 2012, 2013, 2014, 2015, 2016, 2017, 2018,2019,2020]& 	1(0.06\%) \\\hline
10&[2012, 2013, 2014, 2015, 2016, 2017, 2018, 2019, 2020, 2021]& 	4(0.27\%)\\\hline
11&[2011, 2012, 2013, 2014, 2015, 2016, 2017, 2018,2019,2020,2021]& 	2(0.13\%) \\\hline
12&[2010, 2011, 2012, 2013, 2014, 2015, 2016, 2017, 2018,2019,2020,2021]& 116(7.96\%)\\\hline
13&[2009, 2010, 2011, 2012, 2013, 2014, 2015, 2016, 2017, 2018,2019,2020,2021]&99(6.79\%)\\\hline
14&[2008,2009,2010, 2011, 2012, 2013, 2014, 2015, 2016, 2017, 2018,2019,2020,2021]&57(3.91\%)\\\hline
15&[2007,2008,2009,2010, 2011, 2012, 2013, 2014, 2015, 2016, 2017, 2018,2019,2020,2021]&71(4.87\%)\\\hline
16&[2006,2007,2008,2009,2010, 2011, 2012, 2013, 2014, 2015, 2016, 2017, 2018,2019,2020,2021]&157(10.77\%)\\\hline
\bottomrule
\end{tabular}
}}
\caption{Toxic users}
% \vspace{-2mm}
\label{tab:consecutive_year_toxic}
\end{table}
%-
%%
\begin{table}[]
\centering
\resizebox{0.30\textwidth}{!}{
{\large
\begin{tabular}{l|r|r}
\toprule
{\bf \#years}& {\bf \#timelines}&{\bf \# users}\\
\midrule
1& [2021]&1,011(9.42\%)\\\hline 
1& [2020]&90(0.83\%)\\\hline 
1& [2019]& 127(1.18\%)\\\hline 
1& [2018]& 7(0.06\%)\\\hline 
1& [2017]& 13(0.12\%)\\\hline 
1& [2016]& 1(0.009\%)\\\hline 
2&  [2020, 2021]& 3,989(37.18\%) \\\hline
2& 	[2019, 2020]& 548(5.10\%) \\\hline
2& 	[2018, 2019]& 362(3.37\%)\\\hline
2& [2017, 2019]& 2,196(20.47\%)\\\hline
2& [2016, 2018]& 1,230(11.46\%) \\\hline
3&[2015, 2016, 2017]& 	440(4.10\%) \\\hline
3&[2014, 2016, 2018] &	329(3.06\%)\\\hline
3&[2016, 2018, 2020]& 	102(0.95\%) \\\hline
3&[2017, 2018, 2020]&	3(0.02\%)\\\hline
3&[2016, 2019, 2020]& 	18(0.16\%)\\\hline
3&[2018, 2020, 2021]& 	261(2.43\%)\\\hline
\bottomrule
\end{tabular}
}}
\caption{Baseline users}
% \vspace{-2mm}
\label{tab:consecutive_year_baseline}
\end{table}
%-
